# Supplementary material for: 3D Shape Augmentation with Content-Aware Shape Resizing
Source: arXiv:2405.09050 source file (2024-05-15)
Supplement: Supplementary file 1 [file appendix.tex]

\begin{appendices}

\section{Additional Data Augmentation Results}

\section{Additional 3D Generation Results}

\section{Limitations and Failure Cases}

\section{User Study Details}

\end{appendices}
